# Supplementary material for: Why Do We Click: Visual Impression-aware News Recommendation
Source: arXiv:2109.12651 source file (2021-09-26)
Supplement: Supplementary file 1 [file 6.Appendix.tex]

\section{Appendix}
\label{sec:appendix}
